# Supplementary material for: GETAM: Gradient-weighted Element-wise Transformer Attention Map for Weakly-supervised Semantic segmentation
Source: arXiv:2112.02841 source file (2022-05-10)
Supplement: Supplementary file 1 [file appendix.tex]

\newpage
% \newpage
\section{Pseudo Label Generation Computation Time Comparison}
In this paper, we propose a fast yet effective pseudo label completion module to generate high-quality pseudo labels.
Most existing WSSS methods adopt a multi-step scheme, which requires training multiple networks and has complex interdependencies among steps.
Contrarily, in an end-to-end framework, we only have to train a single network in one go.
Consequently, in the end-to-end training process, pseudo label generation time is important because we are generating pseudo labels and training the network concurrently, 
a slow pseudo label generation module would largely influence the overall training speed. 
In this paper, we propose a fast but effective method to generate high-quality pseudo labels. 
Except  PAMR \cite{Araslanov_2020_CVPR}, our generation method is simply based on logical operations without any time consuming modules or networks.
To validate that, we present a speed comparison between different pseudo label generation methods.

We test the inference times of pseudo label generation of three methods: our proposed activation aware label completion module, reliable label generation module proposed by RRM \cite{zhang2020reliability},and pure CRF \cite{krahenbuhl2011efficient}.
We test on one Nvidia 2080 Ti GPU card, we randomly run for 100 iterations to obtain total inference time with different batch sizes. 
As shown in Fig.~\ref{fig:pseudo time}, although our pseudo labels have higher quality as presented in Table 1 of main paper, 
our activation aware label completion module requires much less time compared to competing methods, which can facilitate a more efficient end-to-end training process.

% \section{More Qualitative Results}

\begin{figure}[!t]
   \begin{center}
   {\includegraphics[width=1\linewidth]{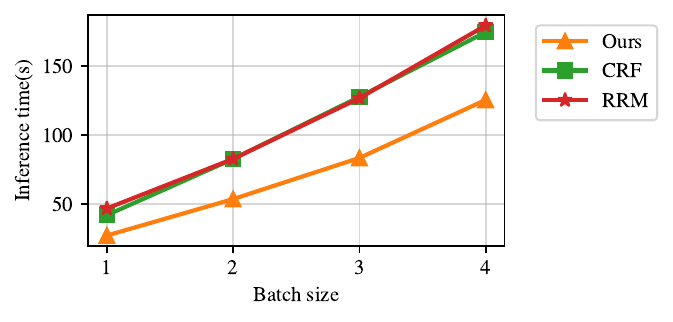}} 
   \end{center}
\caption{Comparison of inference time of different pseudo label generation methods. The times are computed by the sum of 100 training iterations.}
\vspace{-2mm}
   \label{fig:pseudo time}
\end{figure}

\begin{figure*}[!t]
   \begin{center}
   {\includegraphics[width=1\linewidth]{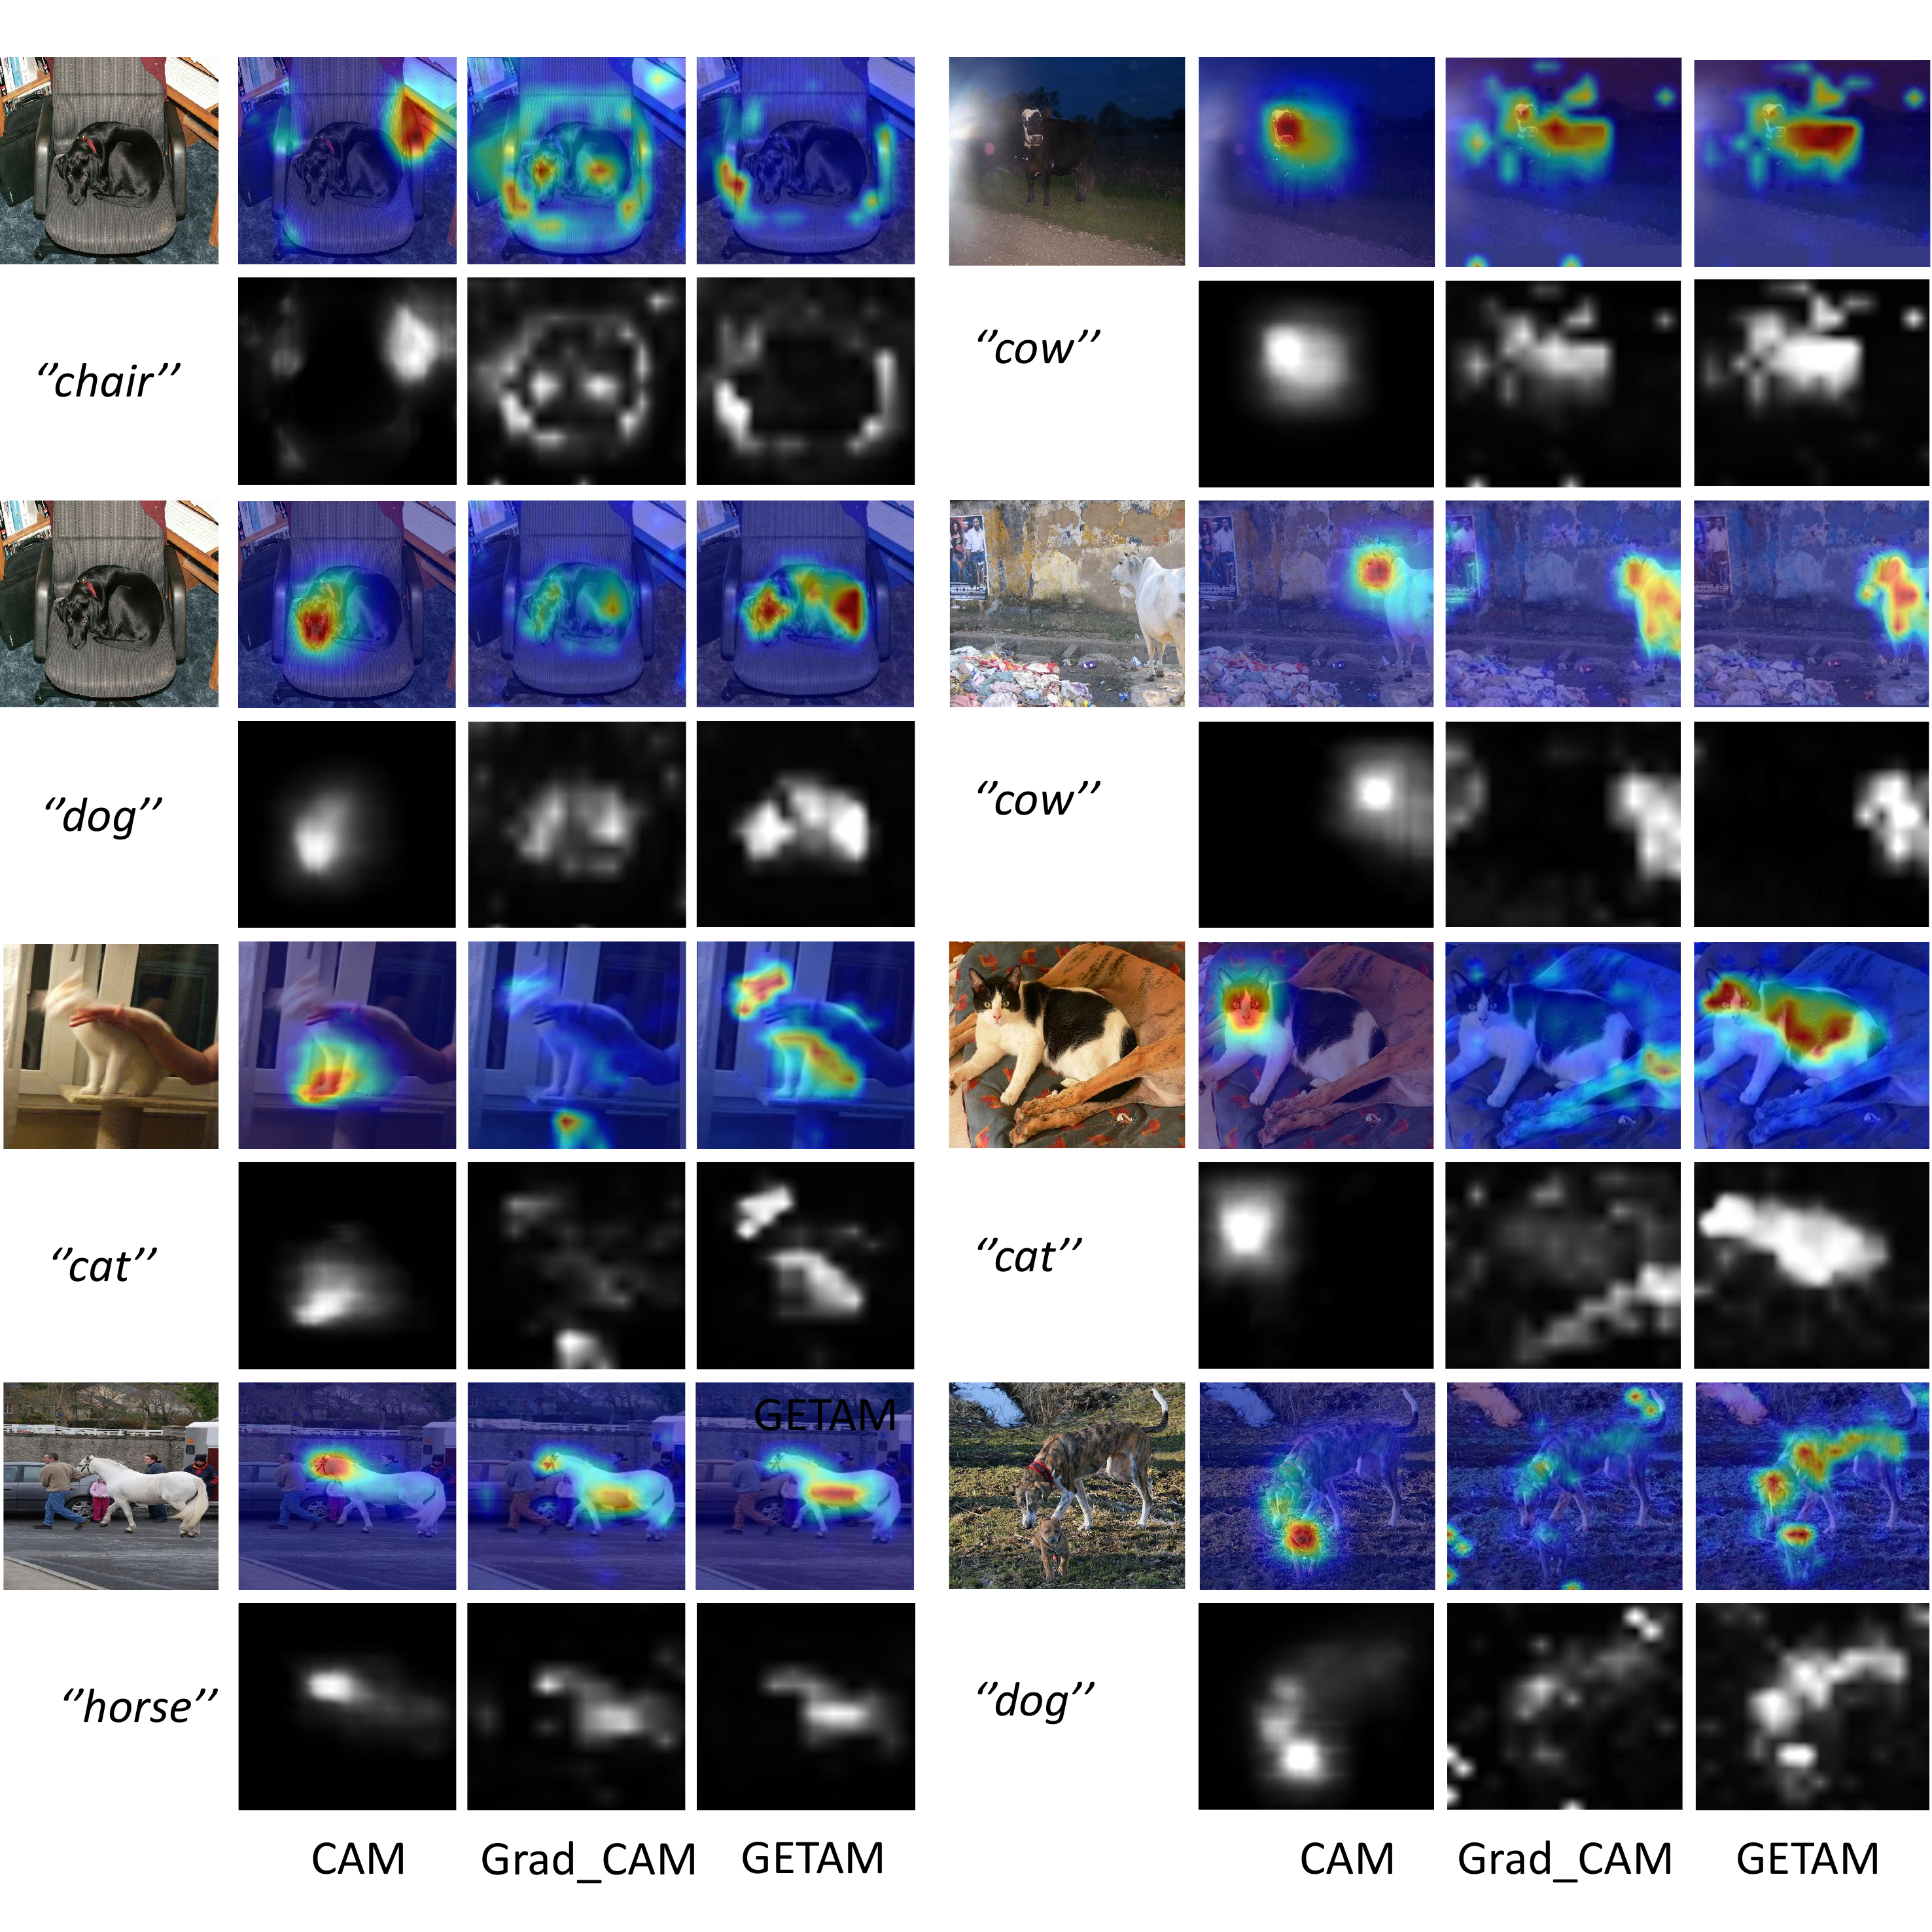}} 
   \end{center}
\caption{Example images of the proposed GETAM compared to CNN-based CAM \cite{zhou2016learning} and ViT-based Grad-CAM \cite{selvaraju2017grad}. As discussed in Section 3, naively migrating CAM to vision transformers results in poor results. So we show baseline CAMs obtained from a CNN network, which overly concentrate on discriminative object regions. 
Second, we migrate Grad-CAM \cite{selvaraju2017grad} to vision transformer, which can locate objects but may introduce undesired noise.
We propose GETAM for vision transformers, which can better capture object shapes and suppress noise than regular CAMs.}
\vspace{-2mm}
   \label{fig:supp pseudo}
\end{figure*}

\begin{figure*}[!t]
   \begin{center}
   {\includegraphics[width=1\linewidth]{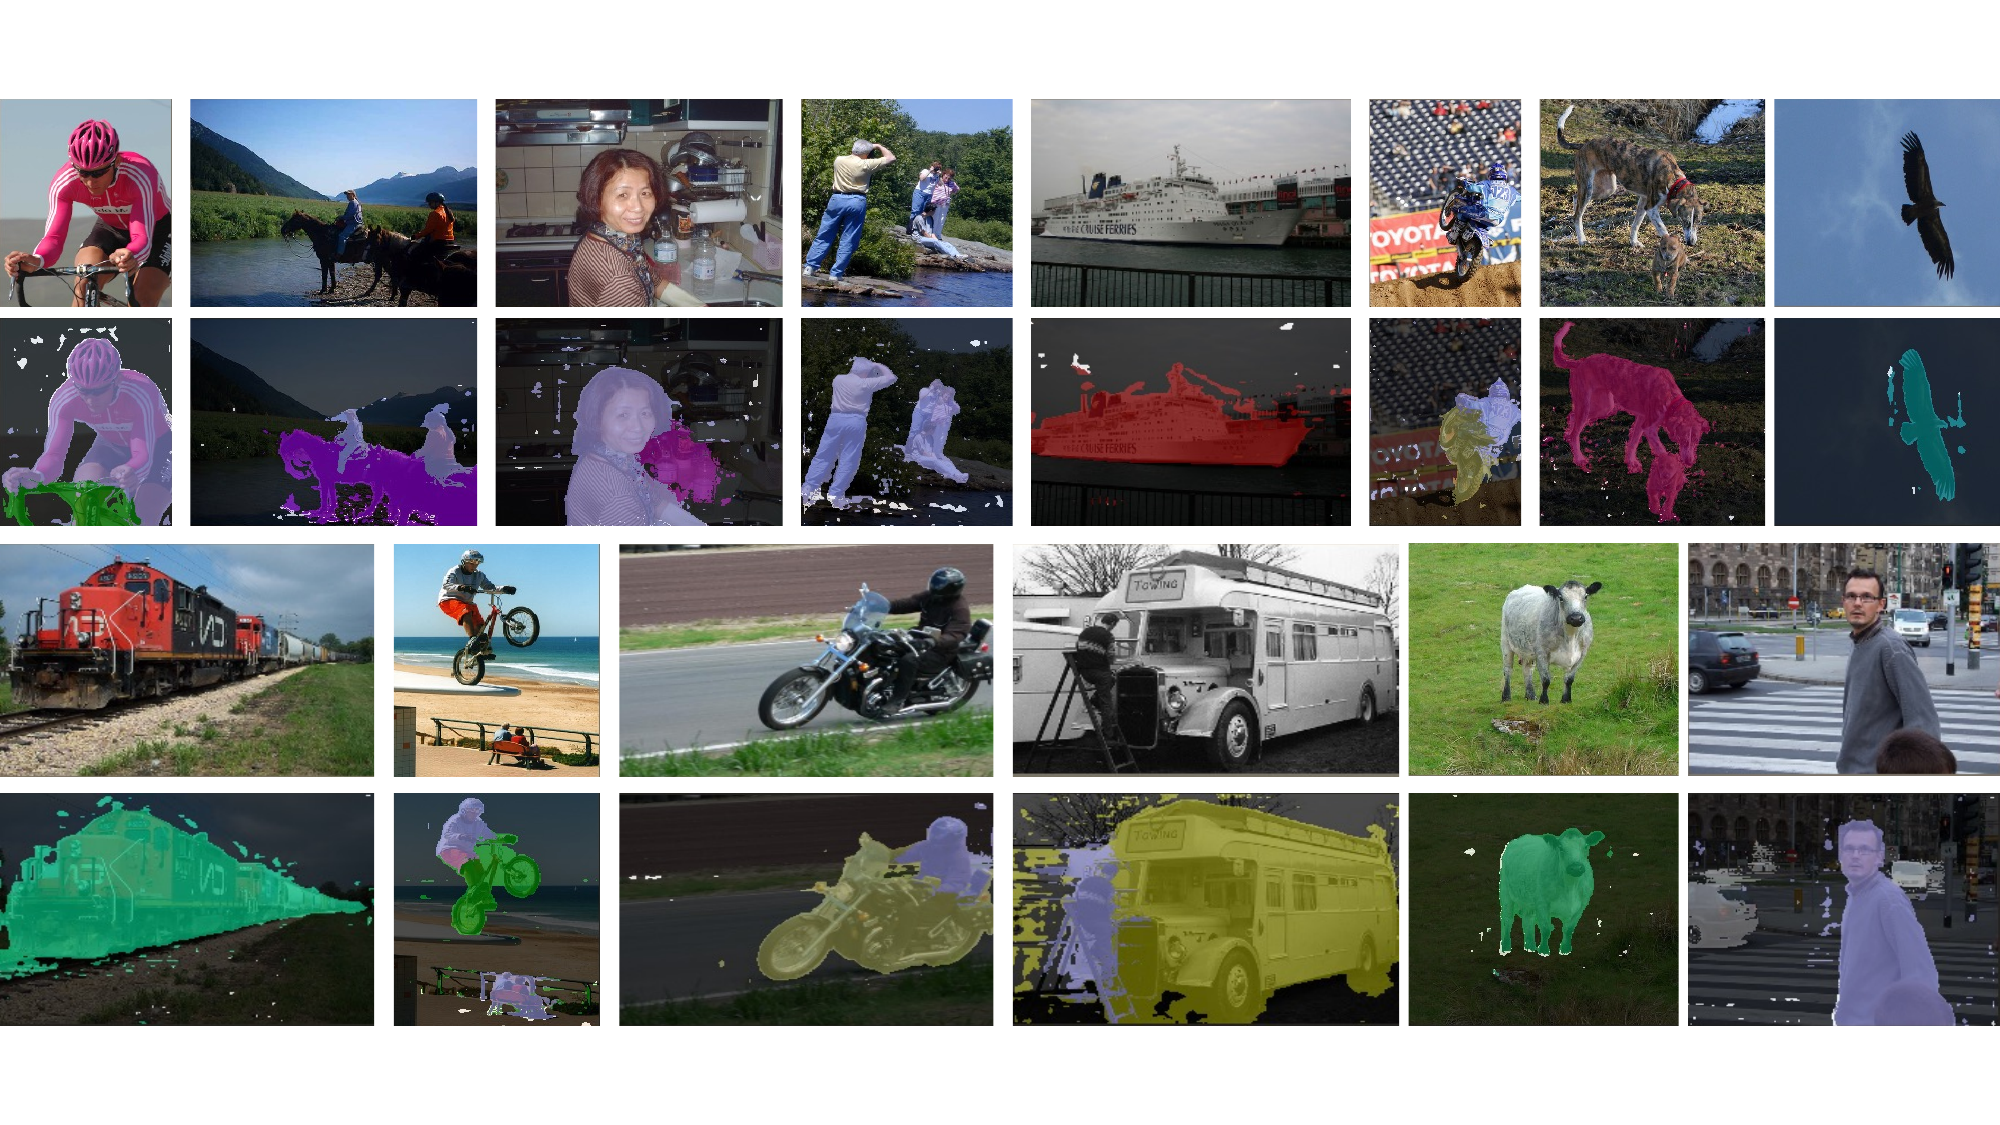}} 
   \end{center}
\caption{More qualitative results of the pseudo labels generated from the proposed approach. Some tiny noisy regions can be observed in the background areas due to the noise of the saliency maps and activation maps. These tiny regions could be simply erased by a image morphological operation, but due to the robustness of our framework, there is no obvious performance improvement.}
\vspace{-2mm}
   \label{fig:supp pseudo}
\end{figure*}

\begin{figure*}[!t]
   \begin{center}
   {\includegraphics[width=1\linewidth]{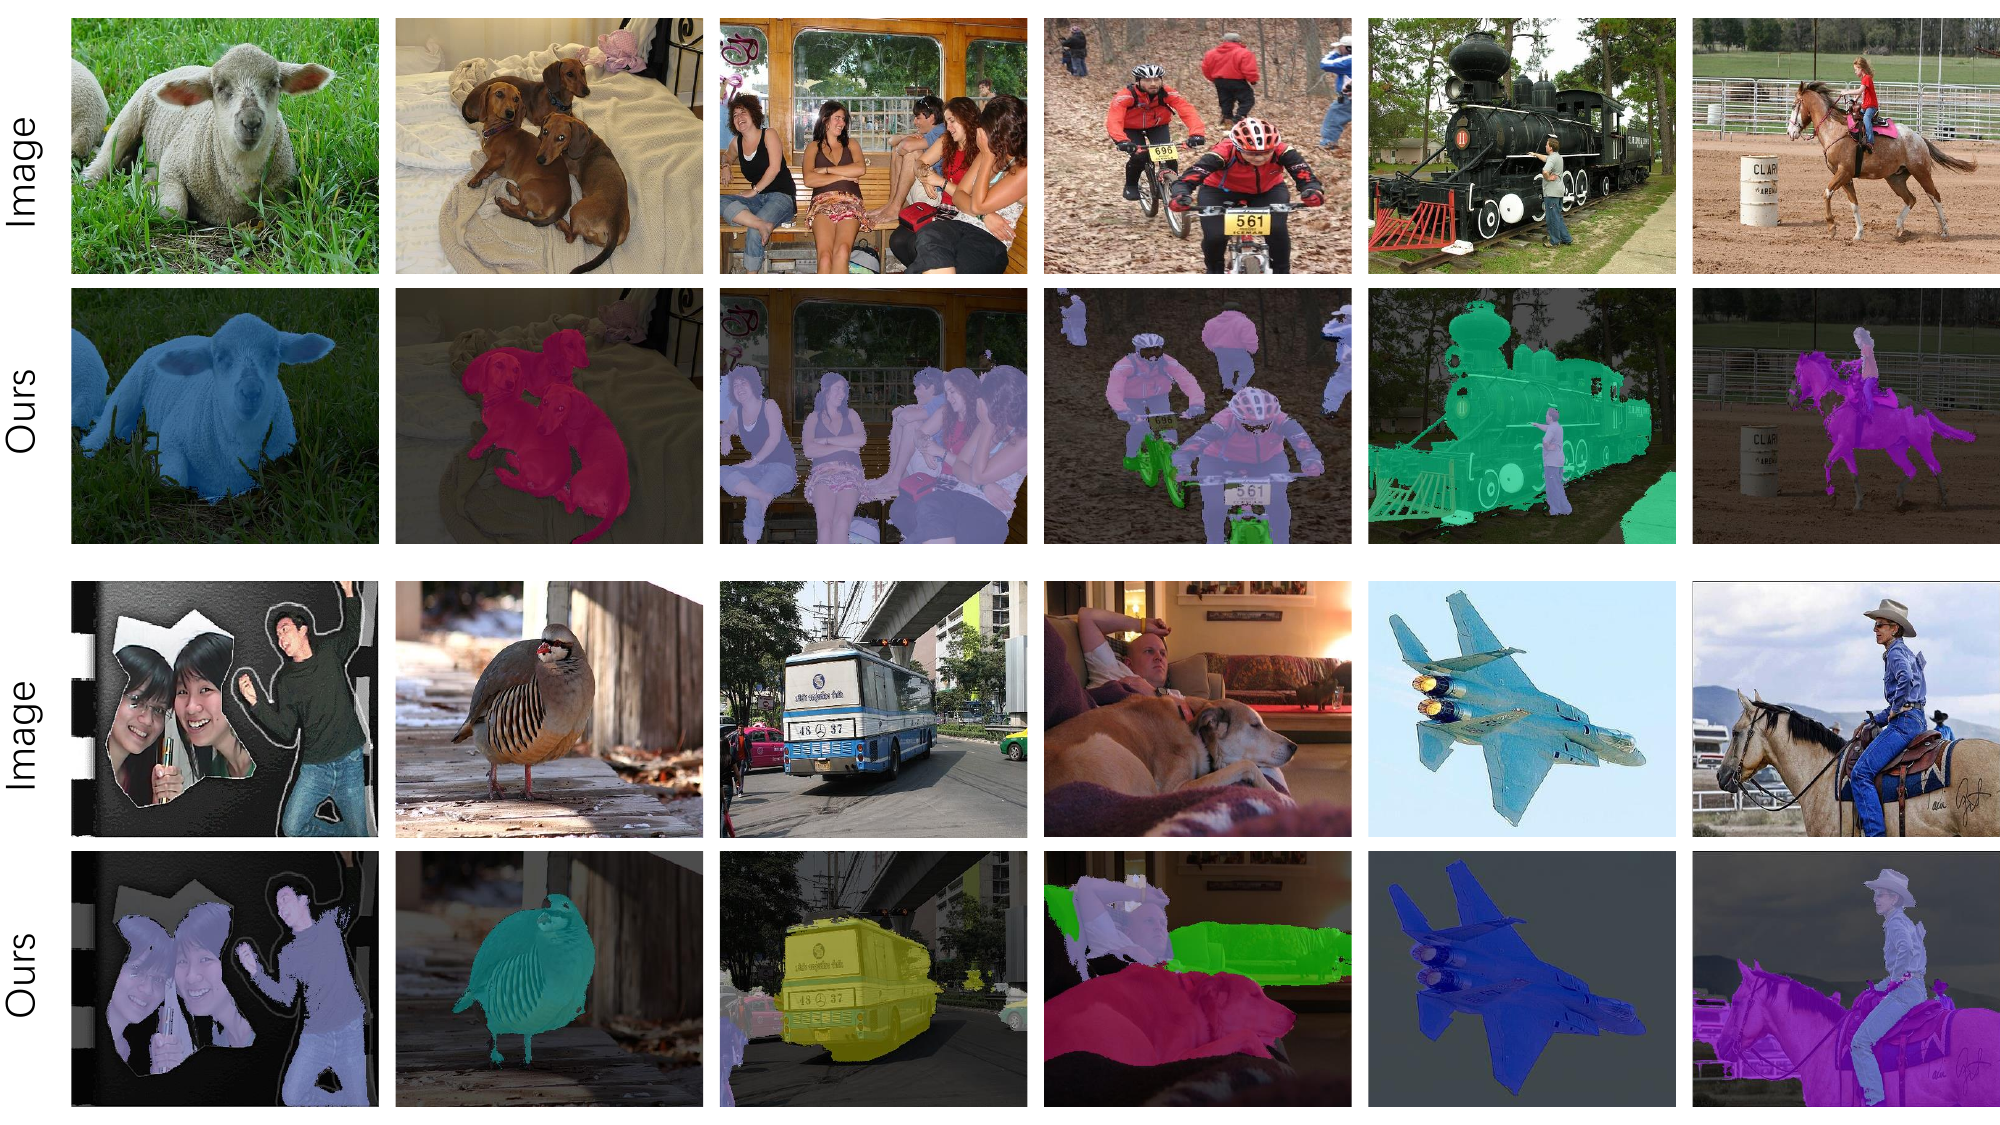}} 
   \end{center}
\caption{Qualitative semantic segmentation results on PASCAL VOC \cite{everingham2010pascal} dataset.}
\vspace{-2mm}
   \label{fig:coco}
\end{figure*}

\begin{figure*}[!t]
   \begin{center}
   {\includegraphics[width=1\linewidth]{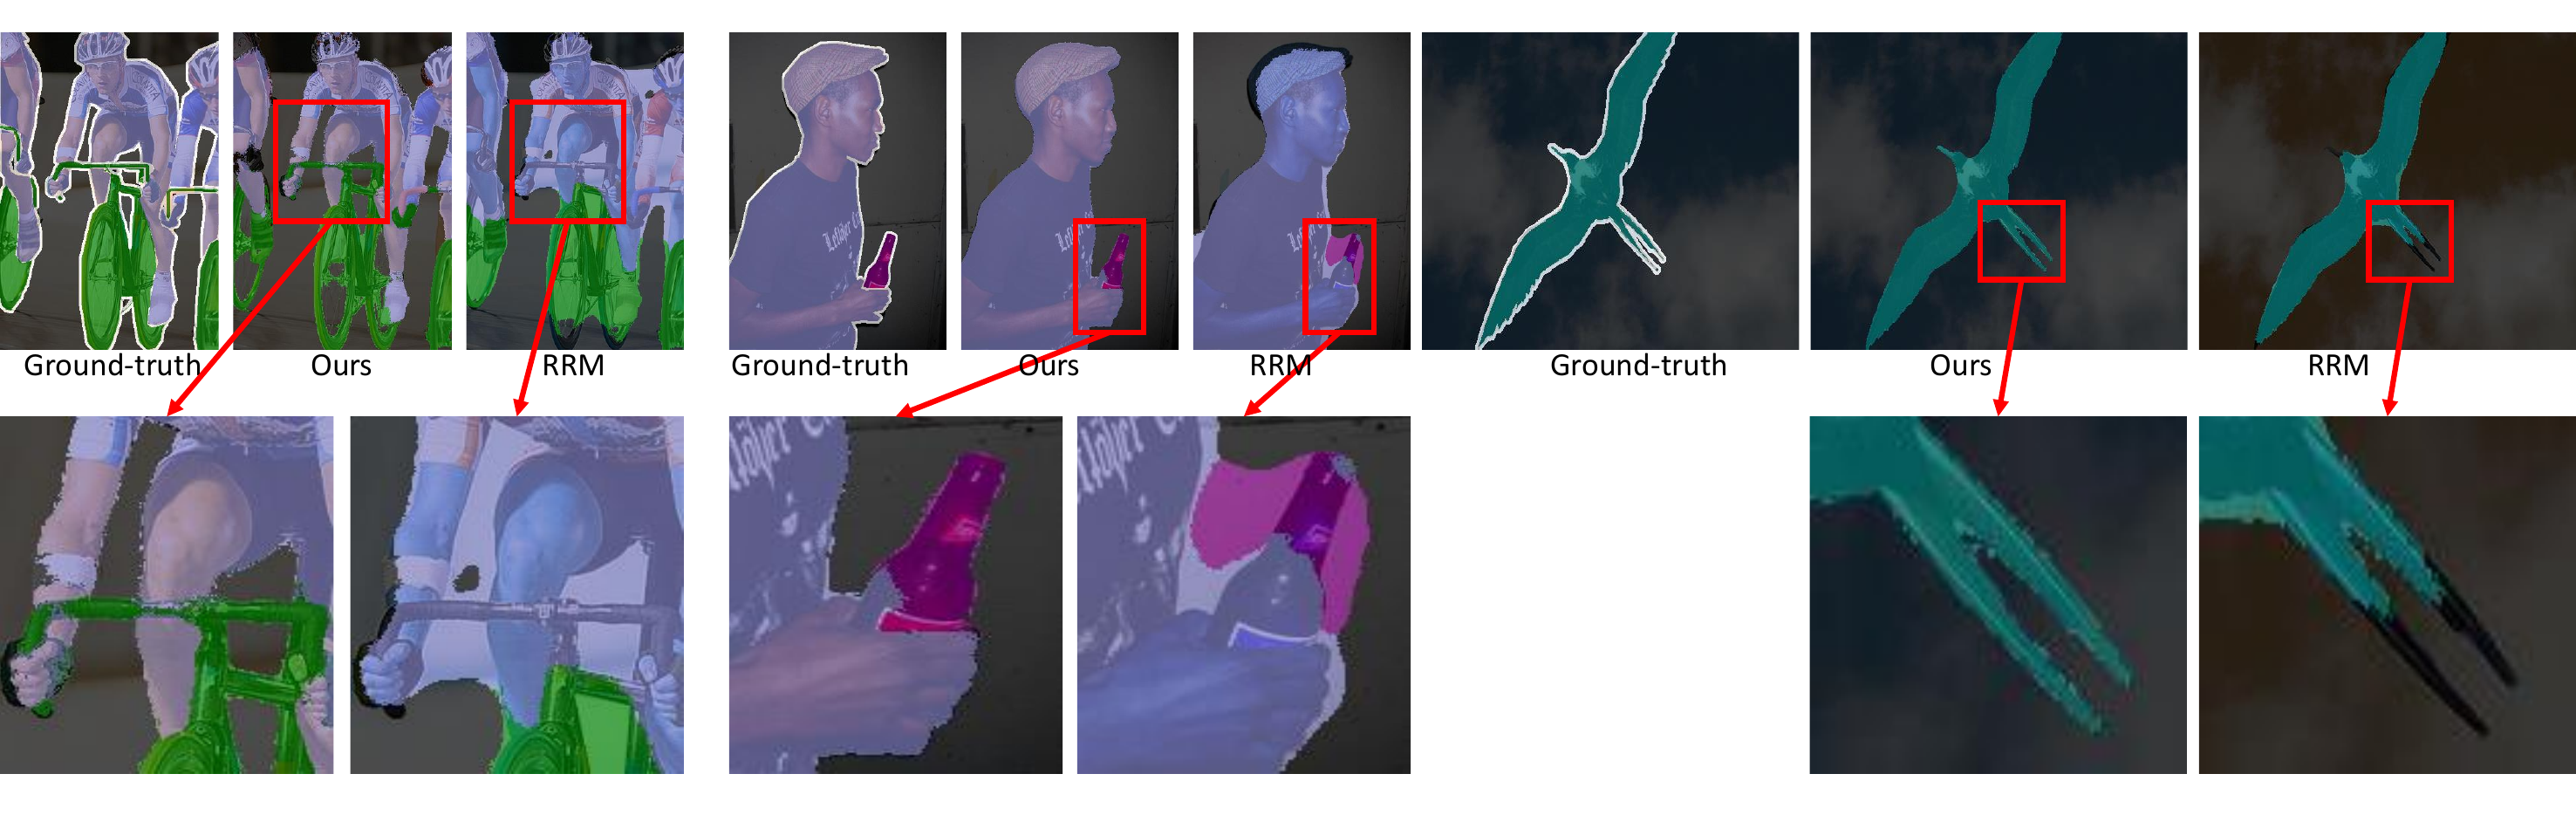}} 
   \end{center}
\caption{Detail comparison of our segmentation predictions compared to our baseline\cite{zhang2020reliability}. 
Due to the proposed GETAM can capture better object shapes, we can generate high-quality pseudo labels and which lead to segmentation predictions with better fine-grained details.}
\vspace{-2mm}
   \label{fig:coco}
\end{figure*}

\begin{figure*}[!t]
   \begin{center}
   {\includegraphics[width=1\linewidth]{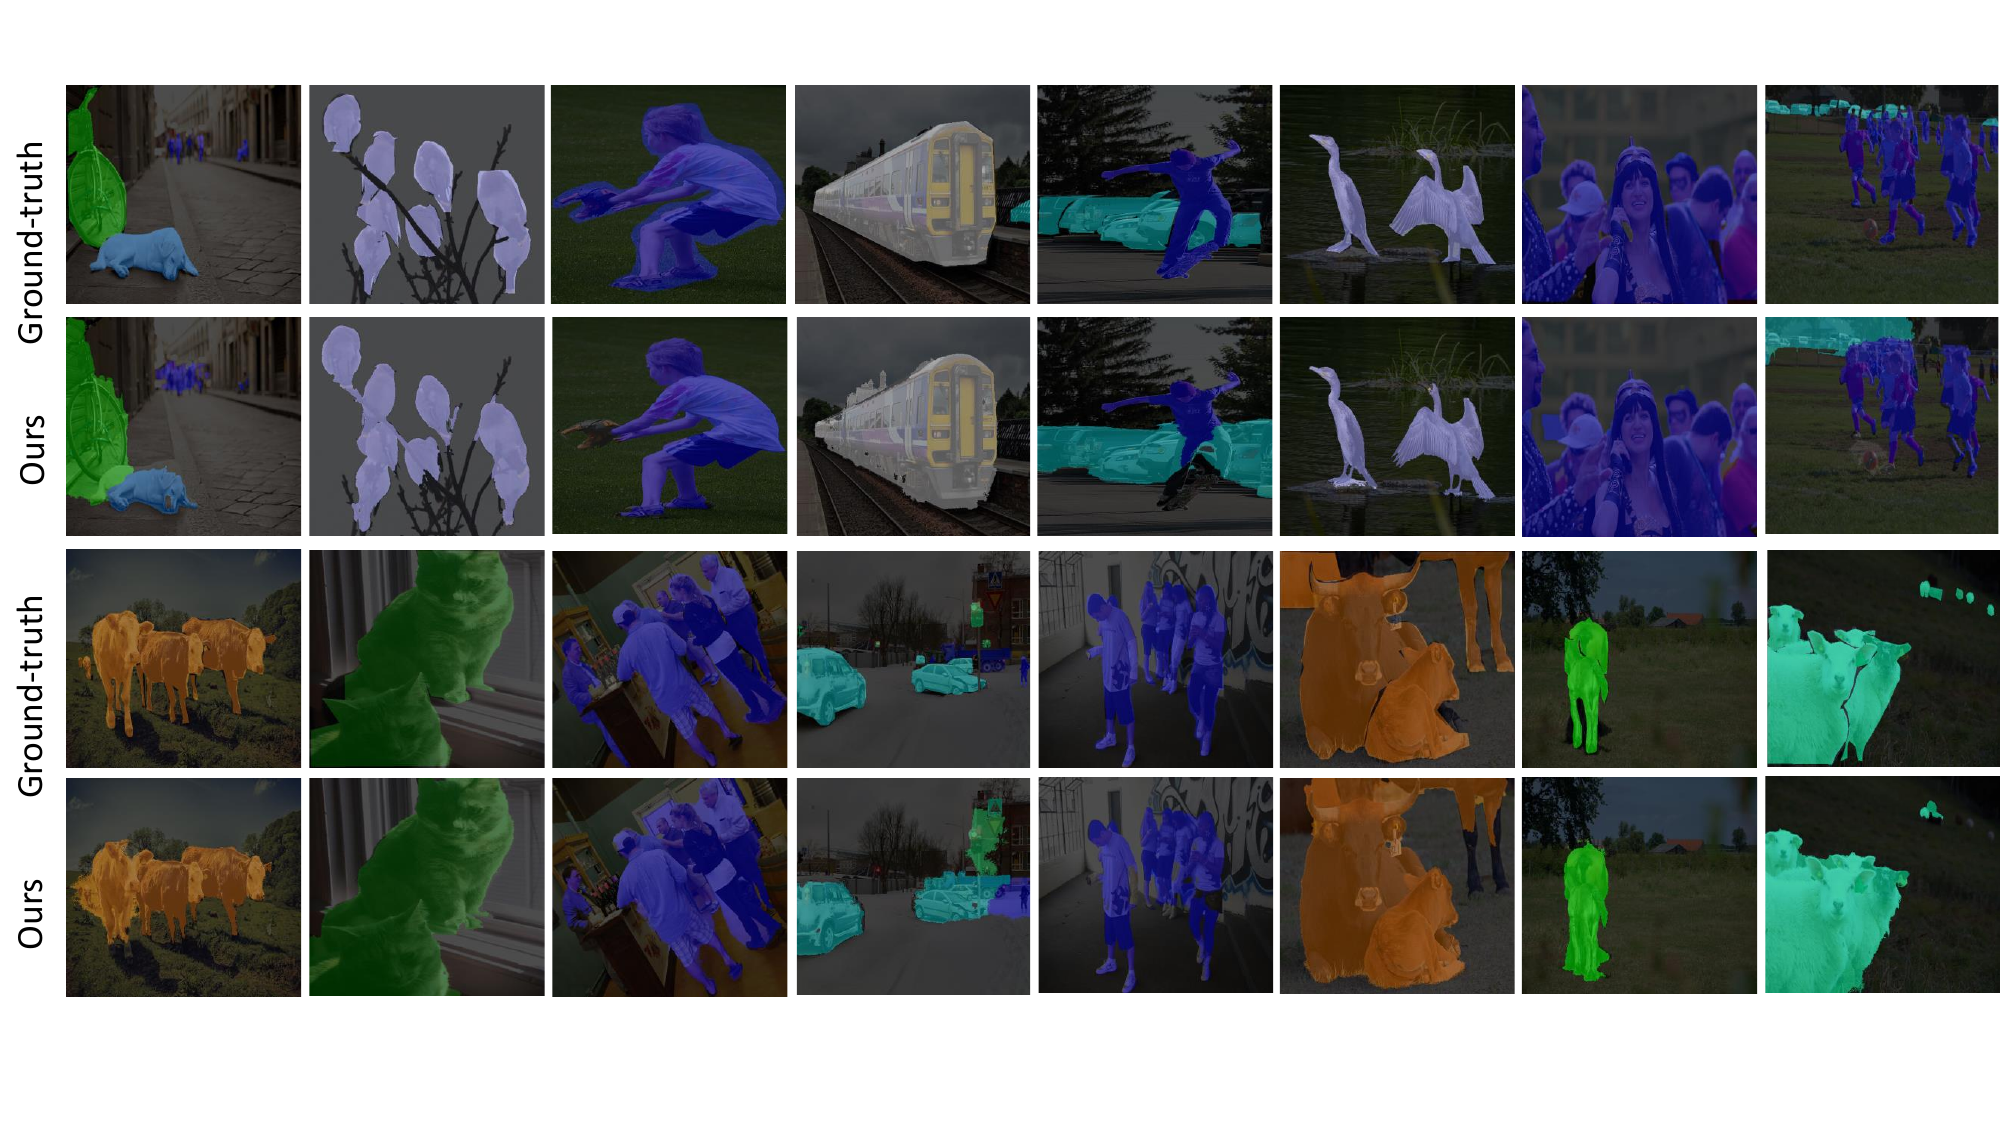}} 
   \end{center}
\caption{Qualitative semantic segmentation results on COCO dataset\cite{lin2014microsoft}. Images from COCO contain multiple objects and more complex scenes, the proposed method can still perform well.}
\vspace{-2mm}
   \label{fig:coco}
\end{figure*}

\section{Ablation: High activation Object Mining}
In the proposed activation aware label completion module, 
we propose to mine highly activated regions in the non-salient regions. 
We argue that since saliency detection models are always trained with foreground objects with center bias, the generated saliency maps on PASCAL VOC may ignore non-salient objects in the background. 
So after saliency constrained masking, we propose to mine the high activation regions in the background, as these high activation regions are likely to be the erased objects. 
We set a threshold $\alpha$, if the activation at a pixel of class $c$ is higher than $\alpha$ percent of all activation of the same object class, we regard it as highly activated and label it as $c$, otherwise as background (0).
However, the high activation in the non-salient regions could also be over activated parts of foreground objects or other activation noise.
We ablate high confidence $\alpha$ in Table \ref{table high confidence threshold}.
A small $\alpha$ means that we only mine a small regions in the background without clear object shape, while a large $\alpha$ means more complete non-salient object shapes but more noise in the pseudo labels. 

Table \ref{table high confidence threshold} demonstrates the results of using high confidence threshold from  $85\%$ to $100\%$.
When $\alpha=100\%$, we do not perform high activation object mining, \ie, all objects in the non-salient regions are erased, we can observe a performance increment of 2.1\% compared to it after utilizing high activation object mining, which validates the effectiveness of the proposed approach.
And when $\alpha=85\%$, we can see a performance downgrade, as too many non-salient regions are mined with a lot of noise.
% We can observe an obvious improvement when we utilize high activation object mining, which validates its effectiveness, and 
We empirically choose $\alpha=90\%$ for best performance.

\begin{table}[]
\footnotesize
\centering
\begin{tabular}{c|c|c|c|c}
\hline
    $\alpha$   & 85\% & 90\% & 95\% & 1  \\ \hline
mIoU &  69.2 & 70.4 & 70.0 & 68.9   \\ \hline
\end{tabular}
\caption{Ablation study for high confidence threshold for non-salient object mining.}
\label{table high confidence threshold}
\end{table}

\section{Ablation: Results without Saliency Map}
Table \ref{table no saliency} shows the effectiveness of our activation aware label completion guided by saliency information. 
Our proposed GETAM approach with double-backward propagation provides reliable class-wise activation maps during end-to-end training. 
However, saliency maps are helpful in our case as transformer activation has high object recall but noisy boundaries.
During end-to-end training,
we follow \cite{ahn2018learning}, and add an arbitrary background on activation maps and feed them to a simple CRF \cite{krahenbuhl2011efficient} to generate pseudo labels, then use these to supervise semantic segmentation.
As shown, using a CRF, we can still obtain reasonable results showing reliability of our framework.
% If we adopt existing pseudo label generation module like \cite{zhang2020reliability},  
However, activation aware label completion assisted by saliency maps, yields significantly improved performance, showing the effectiveness of our proposed pseudo label generation module.

\begin{table}[]
\footnotesize
\centering
\begin{tabular}{c|c|c}
\hline
Method & CRF & Activation Aware Label Completion
      \\ \hline
mIoU  &  55.1 & 70.4    
\\ \hline
\end{tabular}
\caption{Performance comparison of different pseudo label generation methods:  CRF verus our activation aware label completion module, results obtained on ViT-Hybrid \cite{dosovitskiy2020image}.}
\label{table no saliency}
\end{table}

\section{Segmentation Decoder Structure}
In the segmentation branch, we adopt the decoder structure proposed in \cite{ranftl2021vision}. We give a detailed introduction of this segmentation decoder.

In this decoder, a set of tokens from multiple levels of transformer blocks are assembled as the image-like features at various resolutions. 
Since we use the vision transformer backbone with 12 cascaded transformer blocks, we extract the intermediate output features from the four separated layers following \cite{ranftl2021vision}. After obtaining each output features $O\in \mathbb{R}^{(n+1)\times d}$, we first map the $N+1$ tokens to a set of $N$ tokens by projecting the \texttt{CLS} token using an MLP to obtain $O\in \mathbb{R}^{n\times d}$.
Then, since $n$ is input patch size, $n = w\times h$. We reshape the $O\in \mathbb{R}^{n\times d}$ into an image-like representation by placing each token according to the position of its initial patch in the image $O\in \mathbb{R}^{h\times w\times d}$.
With these image-like representation maps from four consecutive layers of the vision transformer backbone, we apply a RefineNet \cite{lin2017refinenet} based decoder structure to combine them. We progressively up-sample the representation by a factor of two in each fusion stage. The output representation size has half the resolution of the input image. 
Then, we input the output representation into a channel attention block proposed by \cite{hu2018squeeze} to obtain final representation output.
Finally, we attach a simple semantic segmentation head to make final predictions.

% Then the feature representations are progressively up-sampled and fused using a RefineNet-based fusion block \cite{lin2017refinenet} and finally fed into the semantic segmentation prediction head.

\section{Subsidiary Saliency Loss}
%NB In our end-to-end training, 
During the second stage of our end-to-end training, our loss is defined as $L =  L_{\text{cls}} + L_{\text{seg}} + L_{\text{sal}}$, where $L_{\text{cls}}$ is multi-label classification loss between the classification predictions and provided class labels. 
For $L_{\text{seg}}$, we adopt the semantic segmentation proposed by \cite{zhang2020reliability}, which consists of 
cross entropy loss between the semantic segmentation predictions and our pseudo labels, and an energy loss which encourages a better predictions at unlabeled areas (255).

For better object shapes, we present a subsidiary saliency loss during the second stage training.
We observe that after pseudo label completion, we can obtain high-quality pseudo labels which can locate objects in both the foreground and background. 
However, due to the high activation object mining, some noise is generated around foreground objects, as these regions are likely to be highly activated.
Since saliency maps are provided which result in accurate object shapes, we adopt saliency maps as a subsidiary supervision to further refine the boundaries of our semantic segmentation predictions.
$L_{\text{sal}}$ is computed as the binary cross entropy loss between the background channels of the predictions and the non-salient regions in saliency maps. Formally, it is defined as:
\begin{equation}
L_{\text{sal}} = \alpha* BCE(Seg\_{pred}\texttt{[0,:,:]}, 1-sal) 
\end{equation}
Where $1-sal$ denotes non-salient maps. $\alpha$ is a tunable weight to control the weight of the $L_{\text{sal}}$ in overall loss. We empirically choose $\alpha=0.1$ so we can refine the foreground objects shape without suppressing background objects.
